# Supplementary material for: A Comparison of First-order Algorithms for Machine Learning
Source: arXiv:1404.6674 source file (2014-04-26)
Supplement: Supplementary file 1 [file supplementary_material.pdf]

In this supplementary material, we show the results of experiments chosen from Yang et al. (2014). In each machining learning problem, we examine two loss functions and two different values of $\lambda$.

## 1. Comparison of Grouped Feature Selection

From Figure 1c and 1d we can see OSGA is slightly better than the others also from about the $100^{th}$ to $1000^{th}$ iteration. However in the later iterations, PD CP outperforms OSGA, FISTA and Fobos. Fobos achieves a convergence rate $O(1/\sqrt{n})$. We observe fluctuations of FISTA since it is not a monotone algorithm. Within $10^6$ iterations only PD CP begin to converge in the absolute-loss case and hinge-loss case. The convergence rate of PD CP is more better than its theory convergence rate.

## 2. Comparison of of Multi-task learning

Figure 2 compares the performances of solvers in the experiment of Multi-Task Learning. Roughly each figure in Figure 2 follows the same pattern. At the beginning, FISTA and PD CP are comparable. From the $1000^{th}$ iteration to about $10000^{th}$ iteration, FISTA needs less number of iterations to reach error tolerance than PD CP. However, in the following iterations, PD CP converges fastest followed by OSGA.

## 3. Comparison of Max-Margin Matrix Factorization/Matrix Completion

Figure 3 shows that PD CP are superior then FISTA and its convergence rate is even better than $O(1/n^2)$. As Figure 3a and 3b shown, PD CP converges to the optimal solution within 8000 iterations. Whereas the other solvers do not reach the optimal solution. From Figure 3c and 3d, we can observe PD CP has a bigger convergence rate than FISTA.

## 4. Smoothing the Non-smooth Functions

We define an absolute value function $F(x) = |x|$. The smooth function we use is

$$F(x) = \begin{cases} \frac{x^2}{2\epsilon} + \frac{\epsilon}{2} & |x| \le \epsilon \\ |x| & \text{otherwise} \end{cases}$$

where $\epsilon \in \mathbb{R}^+$ is a parameter deciding the degree of the smoothness.

For hinge loss, we follow Chapelle (2007). Let a hinge loss be $F(x) = \max(x, 0)$. We define the smooth function as

$$F(x) = \begin{cases} 0 & x < -\epsilon \\ \frac{(x+\epsilon)^2}{4\epsilon} & |x| \le \epsilon \\ x & x > \epsilon \end{cases}.$$

Suppose an insensitive loss $f(x) = \max(|x| - h, 0), h \in \mathbb{R}^+$. We define its smooth function as follows:

$$F(x) = \begin{cases} \frac{(x-h+\epsilon)^2}{4\epsilon} & h-\epsilon < x < h+\epsilon \\ 0 & -h+\epsilon \le x \le h-\epsilon \\ \frac{(-x-h+\epsilon)^2}{4\epsilon} & -h-\epsilon < x < -h+\epsilon \\ |x| - h & x \in [h+\epsilon, +\infty] \text{ or } [-\infty, -h-\epsilon] \end{cases}$$

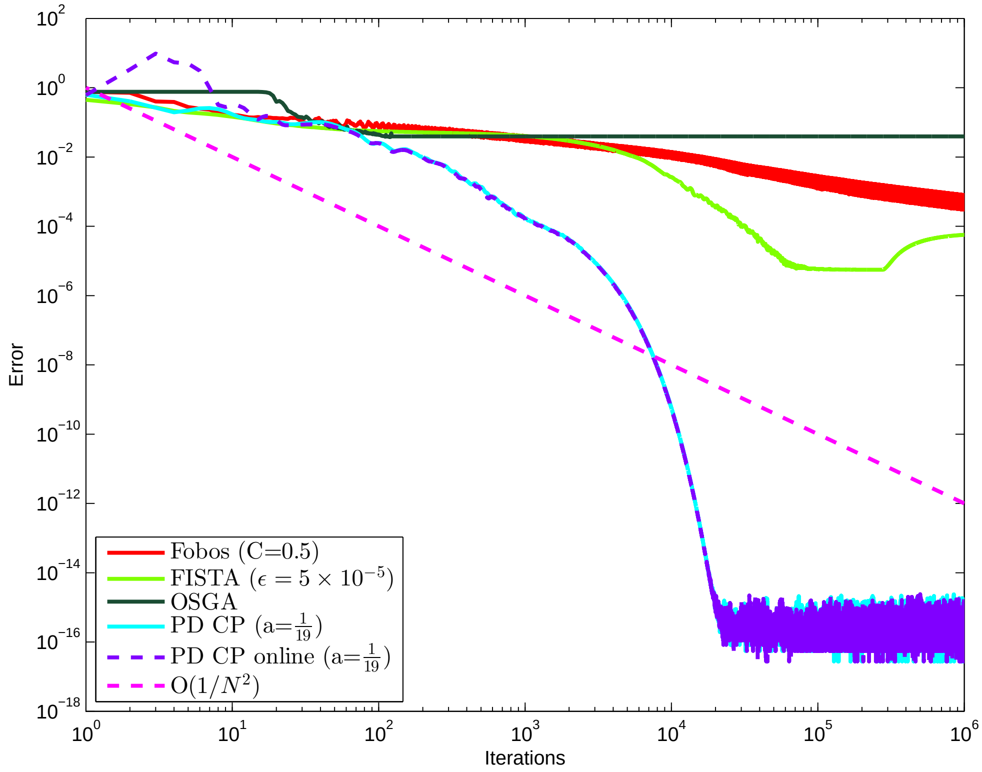


(a) Grouped Feature Selection with the absolute loss using $\lambda = 10^{-3}$

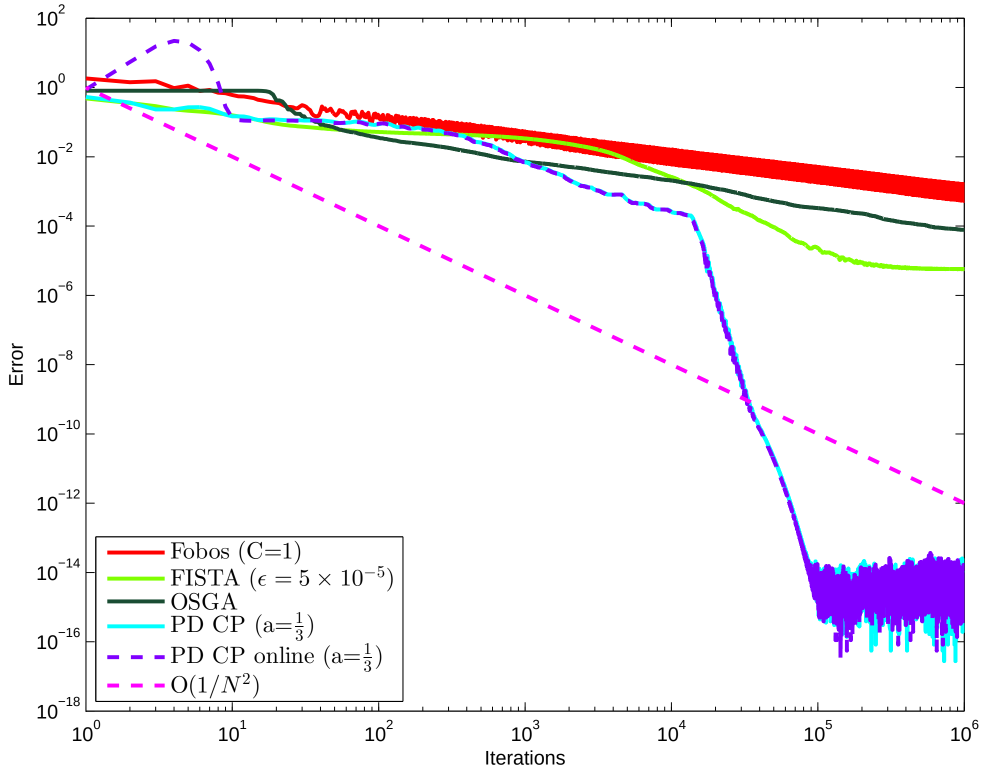


(b) Grouped Feature Selection with the absolute loss using $\lambda = 10^{-5}$

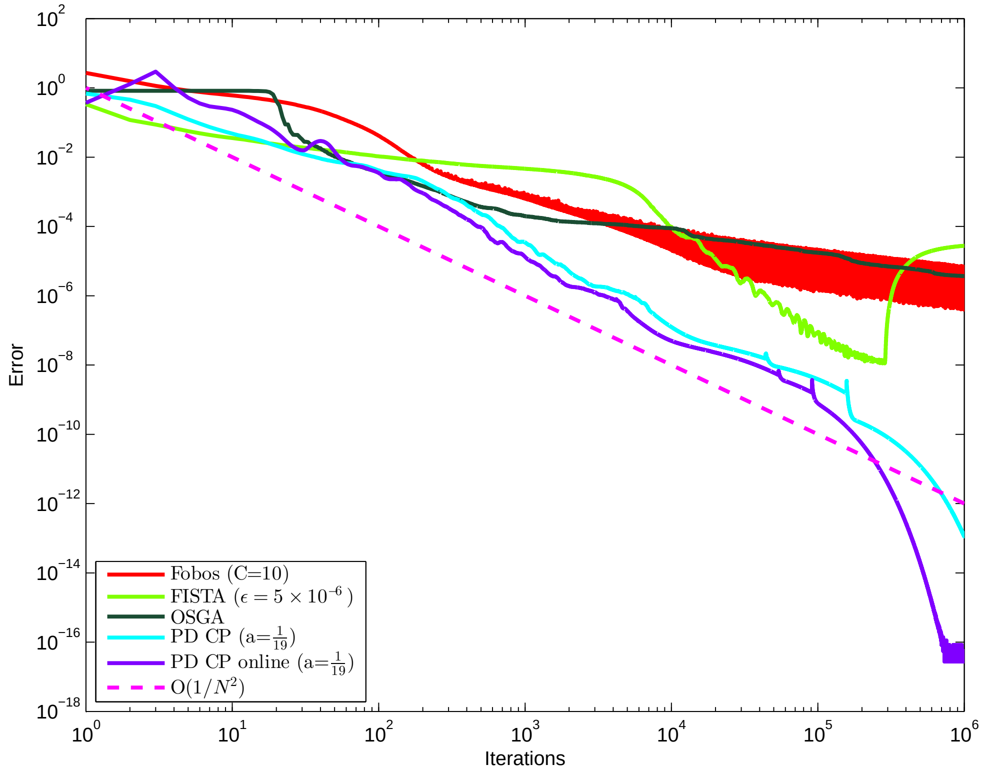


(c) Grouped Feature Selection with the hinge loss using $\lambda = 10^{-3}$

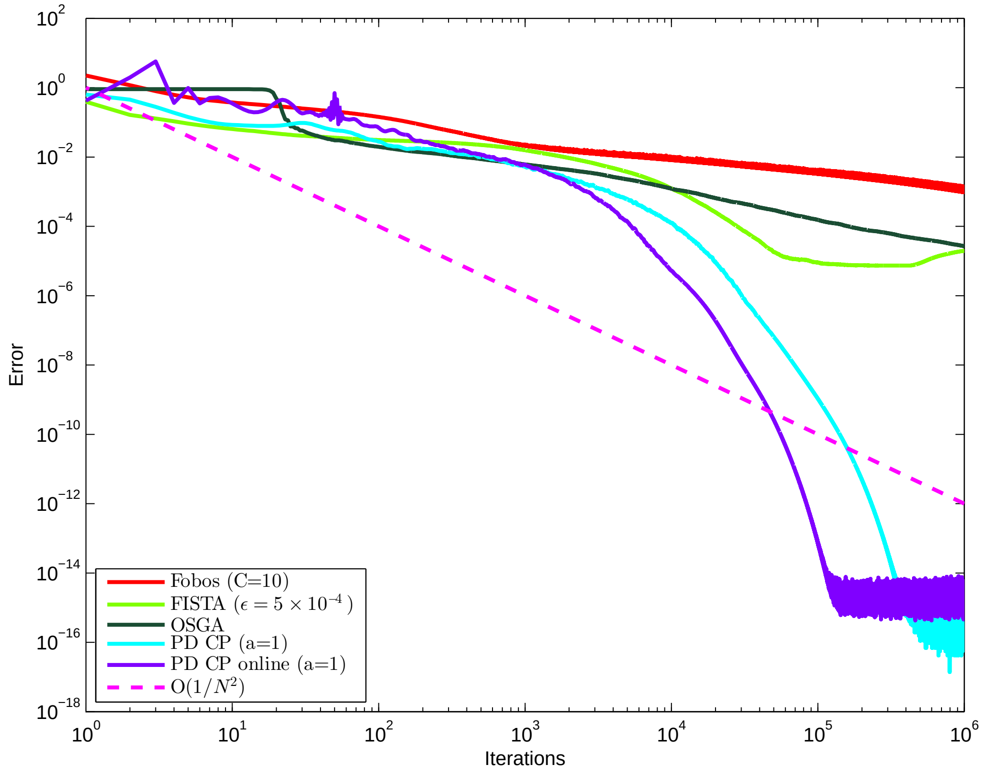


(d) Grouped Feature Selection with the hinge loss using $\lambda = 10^{-5}$

Figure 1: Grouped Feature Selection

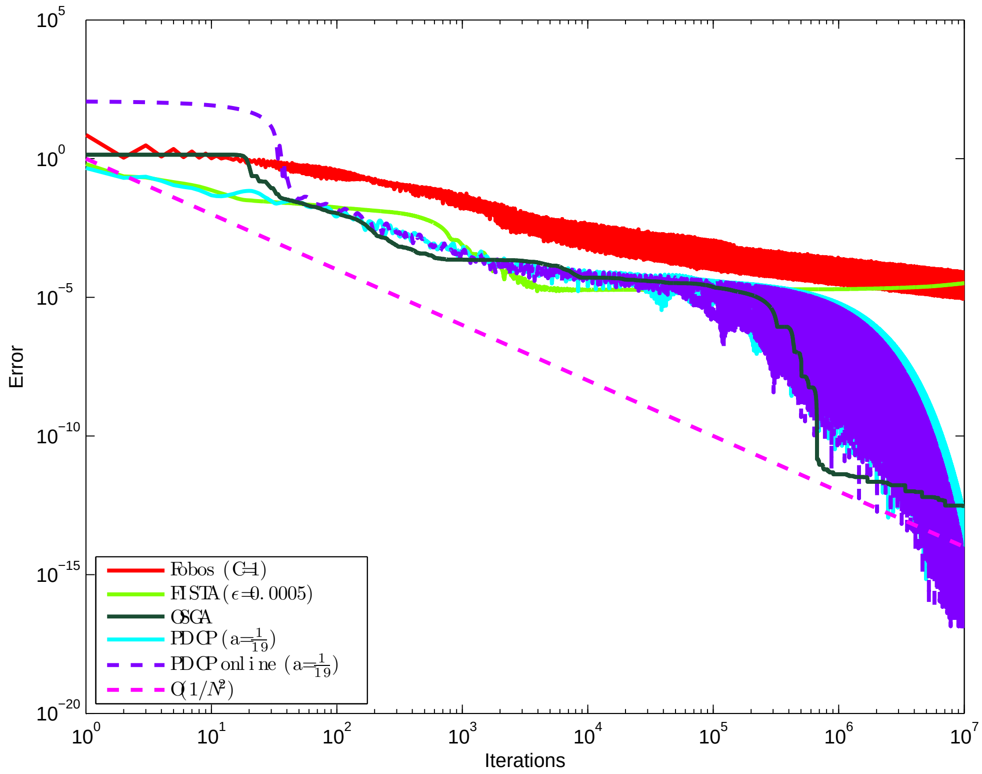


(a) Multi-Task Learning with the absolute loss using $\lambda = 10^{-3}$

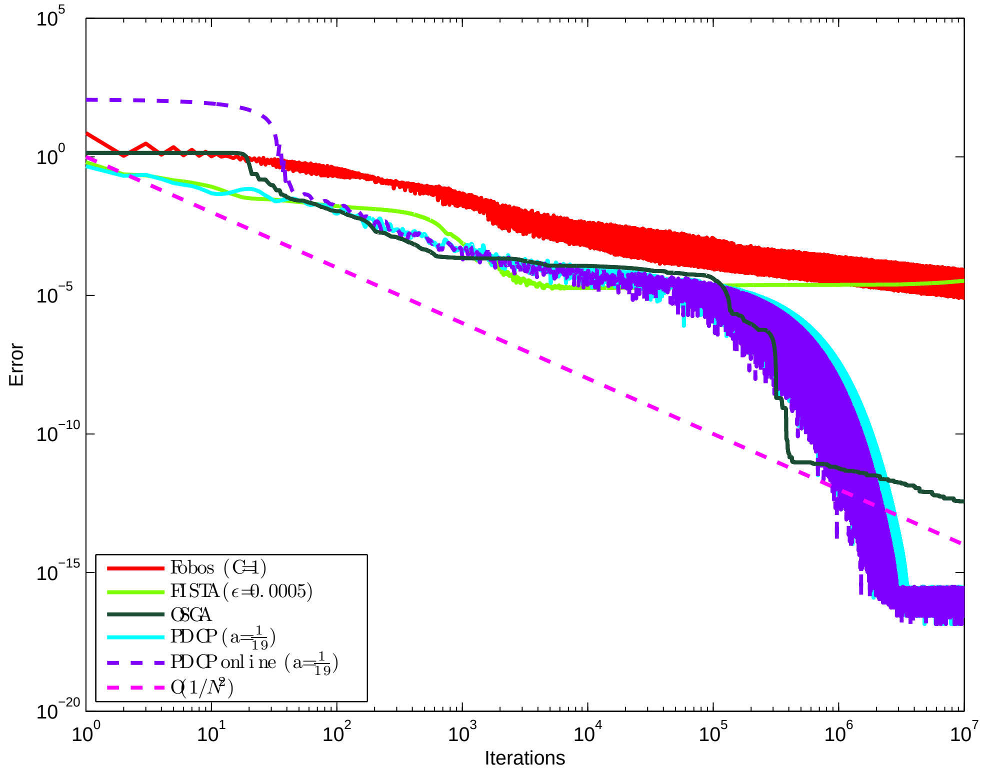


(b) Multi-Task Learning with the absolute loss using $\lambda = 10^{-5}$

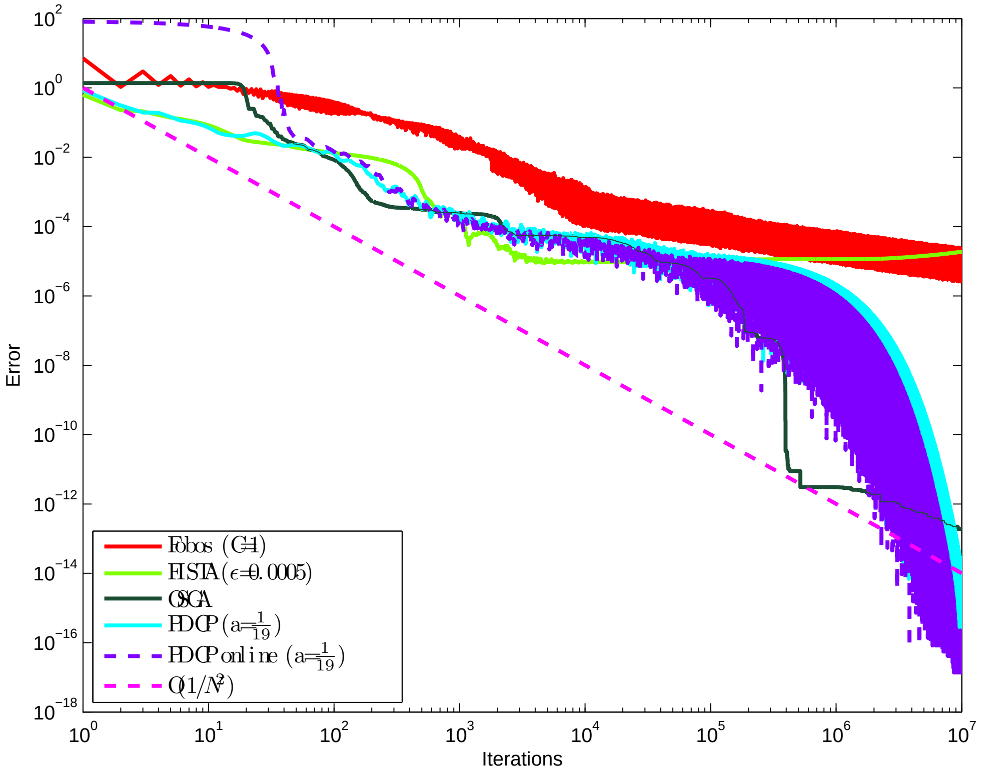


(c) Multi-Task Learning with the insensitive loss using $\lambda = 10^{-3}$

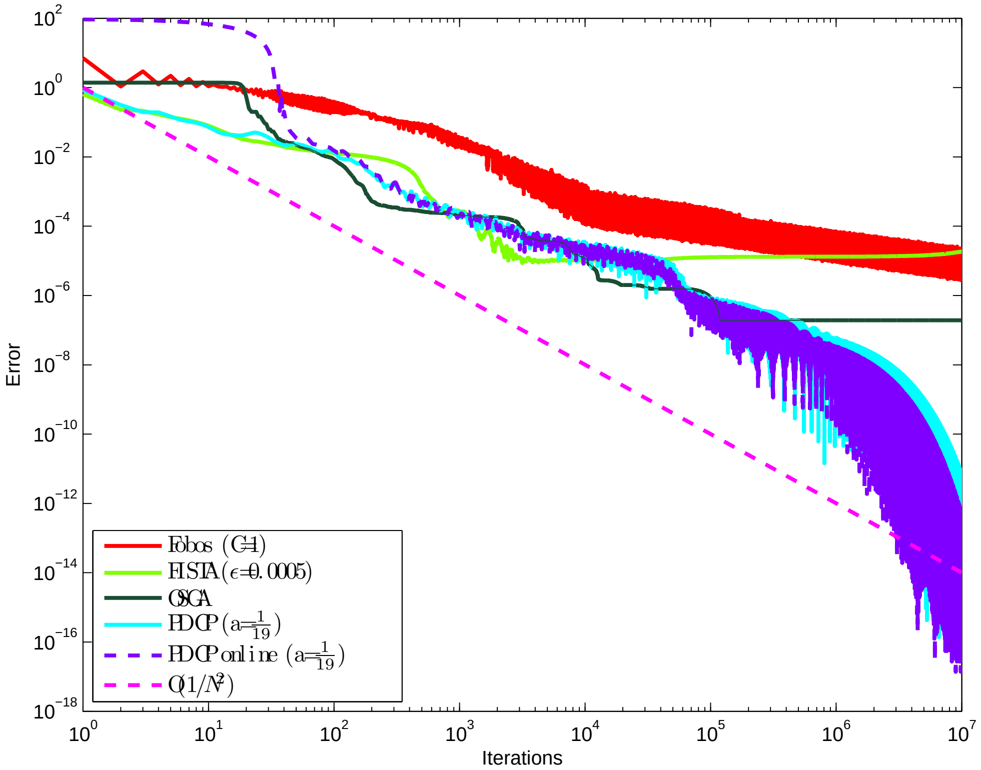


(d) Multi-Task Learning with the insensitive loss using $\lambda = 10^{-5}$

Figure 2: Multi-Task Learning ($\widehat{E}$ are from Online PD CP.)

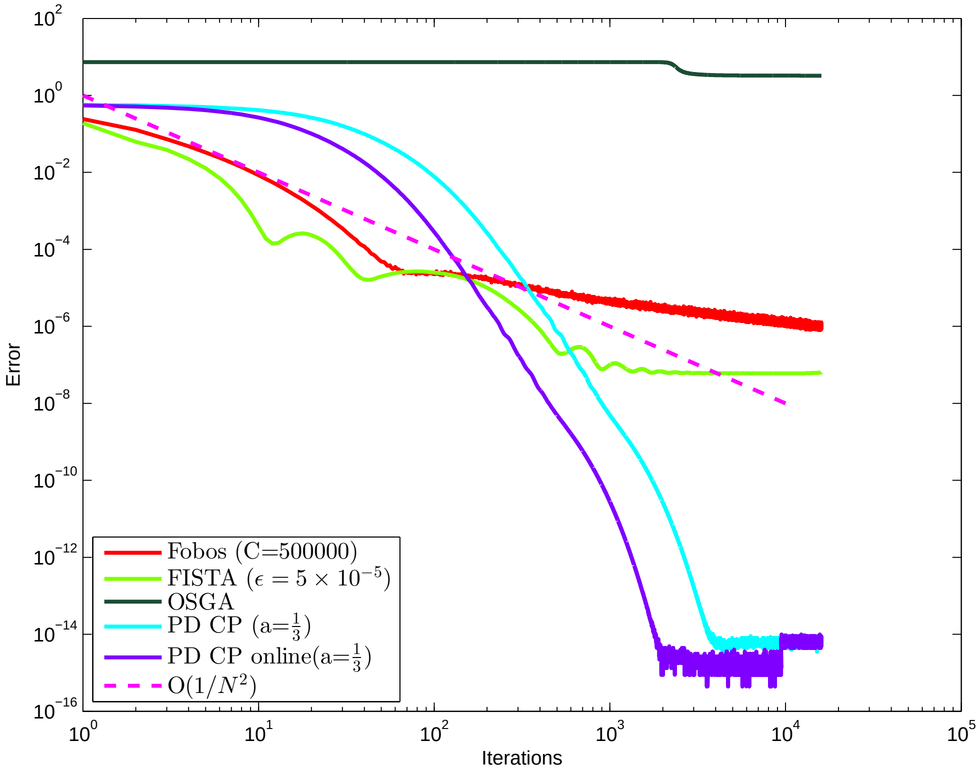


(a) Matrix Completion using $\lambda = 10^{-3}$

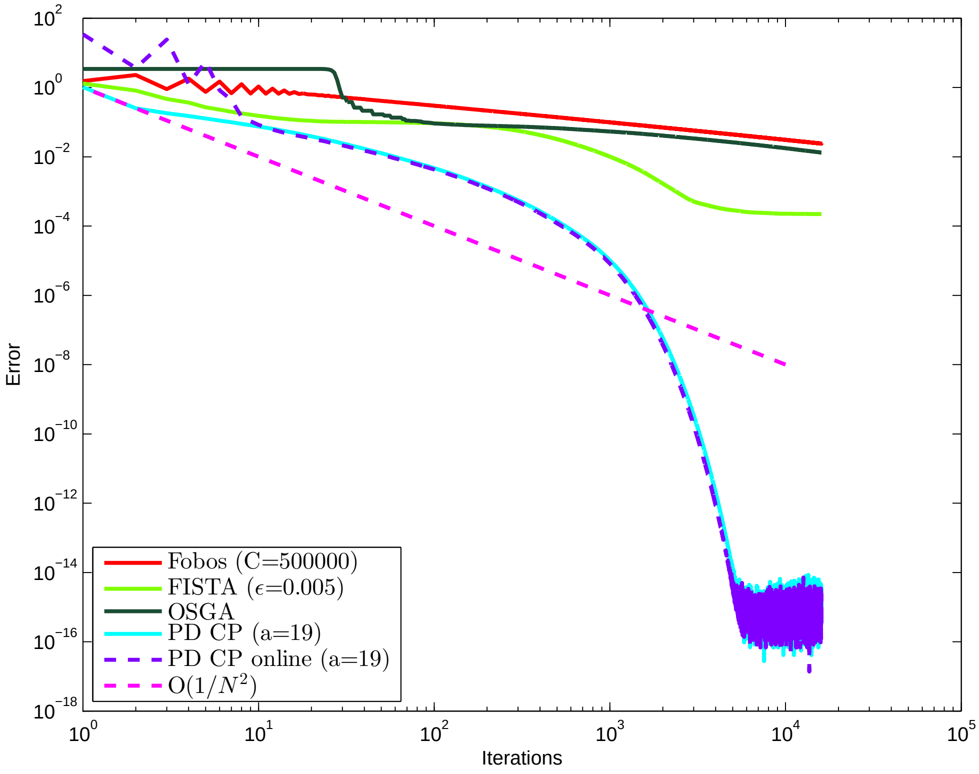


(b) Matrix Completion using $\lambda = 10^{-5}$

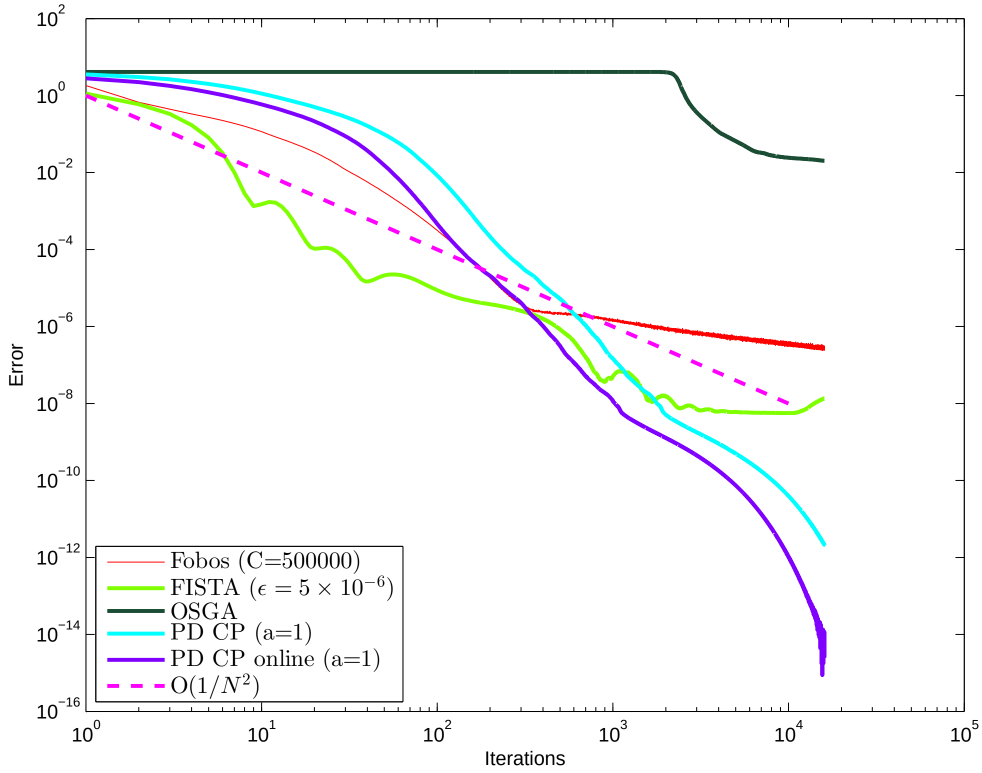


(c) Matrix Factorization using $\lambda = 10^{-3}$

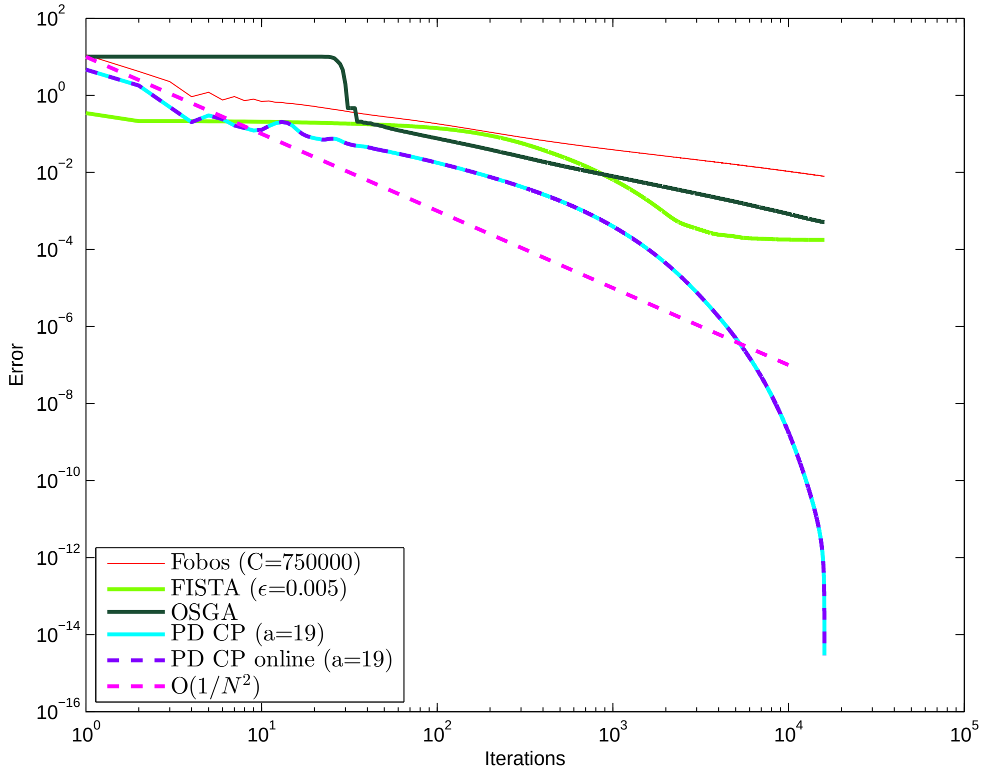


(d) Matrix Factorization using $\lambda = 10^{-5}$

Figure 3: Max-Margin Matrix Factorization/Matrix Completion

where $0 < \epsilon < h$.

## 5. The Proximal Mapping of the Infinity Norm

Let $x, \widetilde{x} \in \mathbb{R}^n$ be two vectors and $G(x)$ be the infinity norm of $x$,

$$G(x) = \max_i |x_i| \,,\ i = 1, \cdots, n$$

where $x_i$ is the $i^{th}$ component of $x$. The Proximal Mapping of the infinity norm $G$, $\mathrm{Prox}_{\lambda\tau\mathrm{G}}(\tilde{x})$ is

$$x = \arg\min_z \left\{ \frac{\|z - \widetilde{x}\|_2^2}{2} + \lambda\tau G(z) \right\}.$$

There are two steps to calculate $x$ based on the following propositions.

**Proposition i** Suppose $G(x) = \omega$, then $x_i = \tilde{x}_i$, $i \in I = \{j : \tilde{x}_j \leq \omega\}$ and $x_k = \omega$, $k \in K = \{j : \tilde{x}_j > \omega\}$.

**Proposition ii** If we randomly change the signs of $\tilde{x}_i$, $G(x)$ does not change and the signs of $x$ should be changed accordingly.

There are two steps to calculate the proximal mapping of the infinity norm. In the first step, we calculate $G(x)$ with the constrain $G(x) = |\tilde{x}_i|$. In this case, $G(x)$ does not change if we remove replicated components in $\tilde{x}$. Thus, we sort $|\widetilde{x}|$ in descending order and remove replicated components if there are replicated components. The new vector is denoted by $\tilde{c}$. According to the Proposition ii,

$$G(\mathrm{Prox}_{\lambda\tau\mathrm{G}}(\tilde{x})) = G(\mathrm{Prox}_{\lambda\tau\mathrm{G}}(\tilde{c})).$$

**Lemma**

We define $G(\mathrm{Prox}_{\lambda\tau\mathrm{G}}(\tilde{c})) = m = c_j$,

$$m = \begin{cases} c_1 & 2\lambda\tau < c_1 - c_2 \\ \min\limits_k c_k & 2\lambda\tau < 2\sum\limits_{i=1}^{i<k} c_i + \max(k-2, 0)(-c_k - c_{k+1}) - 2c_{k+1},\ k \geq 2 \end{cases}.$$

According to Proposition i,

$$x_i = \begin{cases} \mathrm{sign}(\tilde{x}_i) m & |\tilde{x}_i| > m \\ \tilde{x}_i & \text{otherwise} \end{cases}.$$

In the second step, we calculate the exact $G(x)$. There are two cases. One is $G(x)$ should be larger and the other is $G(x)$ should be smaller. We calculate $u = \lambda\tau - \sum\limits_{i=1}^{i<j} c_i + (j-1)c_j$. We define $d$,

$$d = \begin{cases} -u & j = 1 \\ -\frac{u}{k} & u > 0, j > 1 \\ -\frac{u}{l} & u \leq 0, j > 1 \end{cases}$$

where $l$ is the cardinal of $I = \{i |\, |\tilde{x}_i| > m\}$. We define $\widehat{m} = m + d$, then

$$x_i = \begin{cases} \mathrm{sign}(\tilde{x}_i) \widehat{m} & |\tilde{x}_i| > \widehat{m} \\ \tilde{x}_i & \text{otherwise} \end{cases}.$$

## 6. Selecting the parameter of Gaussian kernel

The Gaussian kernel is defined as $k(x_i, x_j) = \exp(-\frac{\|x_i - x_j\|^2}{2\rho^2})$. $\rho$ is the bandwidth parameter to determine the effective dimensionality of the high space. If $\rho$ is too small, overfitting will occur. A real training data set usually contains a lot of samples. If we random choose the value of $\rho$, SVMs may do not work. We define a variable $\nu_{(i,j)}(\rho) = \exp(-\frac{\|x_i - x_j\|^2}{2\rho^2}), i, j = 1, \cdots, N, i \neq j$ with respect to $\rho$. $x_i, x_j$ are a pair of samples in a training data set and there are $M = \frac{N(N-1)}{2}$ pairs. The variance of $\nu$ is,

$$\mathrm{Var}(\nu) = \frac{\sum\limits_{i \neq j} (\exp(-\frac{\left\|x_i - x_j\right\|^2}{2\rho^2}) - \mu)^2}{M}$$

and $\mu = \frac{\sum\limits_{i \neq j} \exp(-\frac{\left\|x_i - x_j\right\|^2}{2\rho^2})}{M}$ is the mean of $\nu$.

The graph of the function Var of argument $\rho$ roughly is a "bell curve". On the left side of the optimal $\rho$, the gradient of Var are positive. By contrast, on the right side of the optimal $\rho$, the gradient of Var are negative. Thus we use bisection method to calculate the optimal $\rho$. The gradient of $\rho$ is,

$$\frac{8}{M\rho^3} \left\{ \sum_{i \neq j} \|x_i - x_j\|^2 \exp(-\frac{\left\|x_i - x_j\right\|^2}{\rho^2}) - \frac{\sum\limits_{i \neq j} \|x_i - x_j\|^2 \exp(-\frac{\left\|x_i - x_j\right\|^2}{2\rho^2}) \sum\limits_{i \neq j} \exp(-\frac{\left\|x_i - x_j\right\|^2}{2\rho^2})}{M} \right\}.$$

In the following, we show the classification result of the synthetic experiments using a bandwidth calculated by this method.

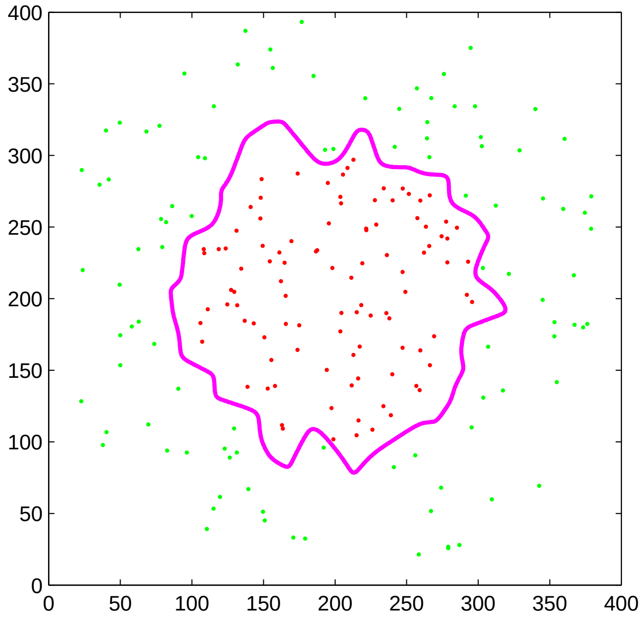


(a) Kernel SVM synthetic experiment 1

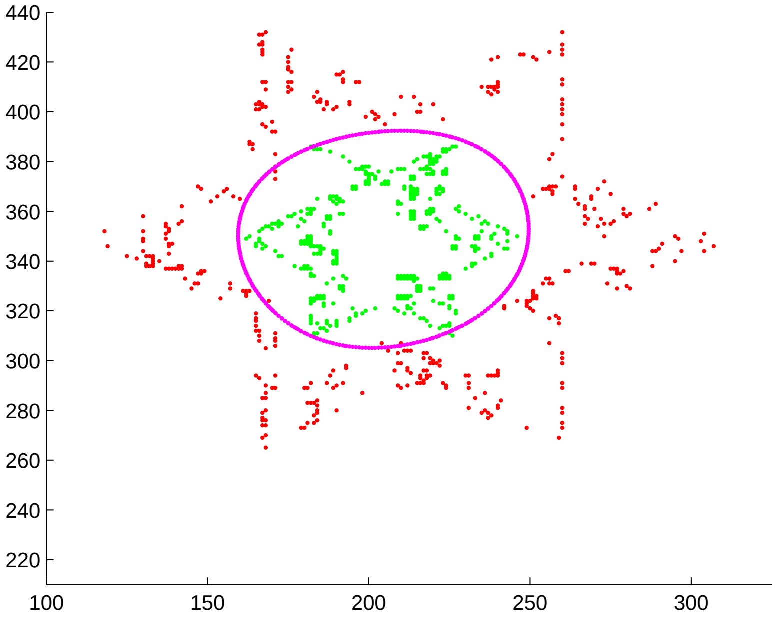


(b) Kernel SVM synthetic experiment 2

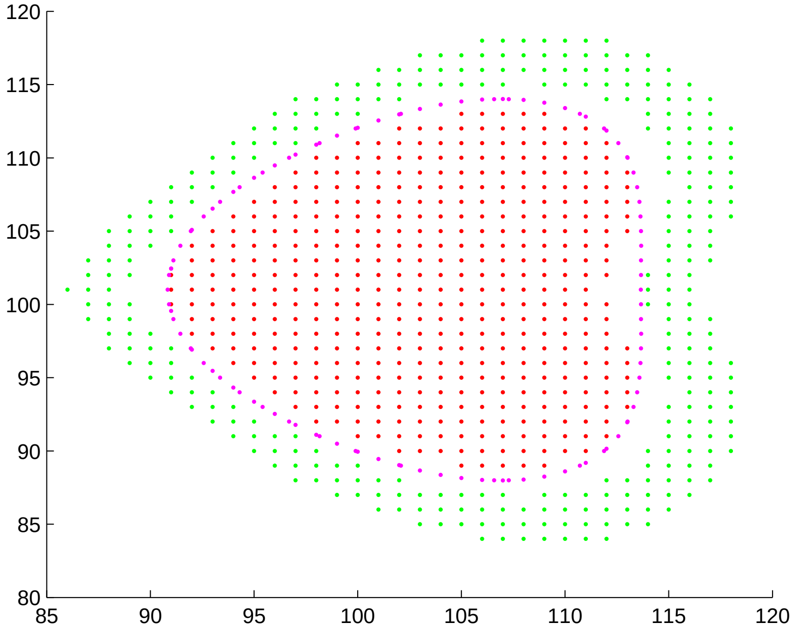


(c) Kernel SVM synthetic experiment 3

## References

Olivier Chapelle. Training a support vector machine in the primal. Neural Computation, 19: 1155–1178, 2007.

Tianbao Yang, Mehrdad Mahdavi, Rong Jin, and Shenghuo Zhu. An efficient primal-dual prox method for non-smooth optimization. Mach Learn, 2014.
